# Supplementary material for: Adaptive Density-Guided Approach to Double Incremental Potential Energy Surface Construction
Source: arXiv:2002.04919 ancillary file (2020-02-12)
Supplement: Supplementary file 1 [file supplementary_material.pdf]

# - Supporting Information -

# Adaptive Density-Guided Approach to Double Incremental Potential Energy Surface Construction

Denis G. Artiukhin[†1], Emil Lund Klinting[†], Carolin König[‖2], and Ove Christiansen[†3]

[†] Department of Chemistry, Aarhus Universitet, DK-8000 Aarhus, Denmark

[‖] Institute of Physical Chemistry, Christian-Albrechts-University Kiel, Max-Eyth-Straße 1, D-24118 Kiel, Germany

Date: February 12, 2020

.

[1]Email: artiukhin@chem.au.dk

[2]Email: koenig@pctc.uni-kiel.de

[3]Email: ove@chem.au.dk

# S1 Determination of Correct Grid Boundaries

Initial computations of 1M2F PESs (for effective FCRs applied, see Tab. S1 in the SI) employing the DIF-ADGA required an unexpectedly large number of SP calculations for convergence. The number of required SPs reached 1580, 5271, and 10735 for the dicyclopropyl ketone, tetraphenyl, and hexaphenyl molecules, respectively. These are about 21.9, 18.3, and 18.3 SPs, on average per vibrational mode, respectively. The use of the DIF-Static scheme led to 1441, 5761, and 11761 SPs for these molecules, i.e., 20 SPs per mode in all three cases. Hence, computational savings were found to be very modest, while applying the ADGA instead of the static grid approach. Moreover, in the case of dicyclopropyl ketone the DIF-ADGA turned out to be computationally more expensive. A closer analysis of the calculated 1M2F PESs revealed that the initial default ADGA boundaries set in relation to the HO quantum number $v = 2$, which has successfully been used in previous non-fragmented ADGA calculations, are too narrow for most of the one-mode cuts. Although the DIF-ADGA was able to determine the correct boundaries in all cases, the algorithm required too many iterations and additional SPs. Therefore, we assumed that a better guess for the initial DIF-ADGA one-mode boundaries reduces the overall computational cost of the method. To validate this assumption, we carried out calculations of 1M2F PESs for the dicyclopropyl ketone, tetraphenyl, and hexaphenyl molecules choosing the initial boundaries according to HO quantum numbers $v = 2$, 4, 6, 8, and 10. The resulting number of required SPs in these computations are presented in Fig. S1. It can be seen that the total number of SPs greatly decreases for the values of $v$ from 2 to 6 for all three molecules. IC and INTRA modes exhibit similar trends. Therefore, this proves our assumption and shows that broader initial boundaries can indeed lead to considerable computational savings in calculations of 1M2F PESs. The use of HO quantum number $v = 8$ leads to a slight decrease in the number of SPs compared to $v = 6$, whereas more SPs are needed for DIF-ADGA computations

with larger values of $v$. This is probably caused by too wide one-mode initially spanned space, which requires more SPs on average. In the following, we consider the initial guess of $v = 8$ to be optimal and, therefore, set it by default in all subsequent DIF-ADGA calculations. For the choice of $v = 8$, only about 8.4, 7.2, and 6.7 SPs on average per mode are required for dicyclopropyl ketone, tetraphenyl, and hexaphenyl, respectively. This leads to considerable computational savings for 1M2F PESs calculations compared to the DIF-Static scheme, where 20 SPs per mode were used.

Once the correct boundaries for one-mode cuts are determined in the ADGA, these are by default fixed for higher-order MC grids without any further optimization. Therefore, the problem of too narrow initial boundaries described in this section affects only 1M$l$F PESs and, as a result, the use of the optimal value $v = 8$ decreases the computational cost of the 1M$l$F parts only. Because the total number of SPs is strongly dominated by higher-order cut-potentials, these computational savings are often minor for $n$M$l$F PES generations with $n \geq 2$. Still, a good starting guess is essential for both algorithm efficiency and stability.

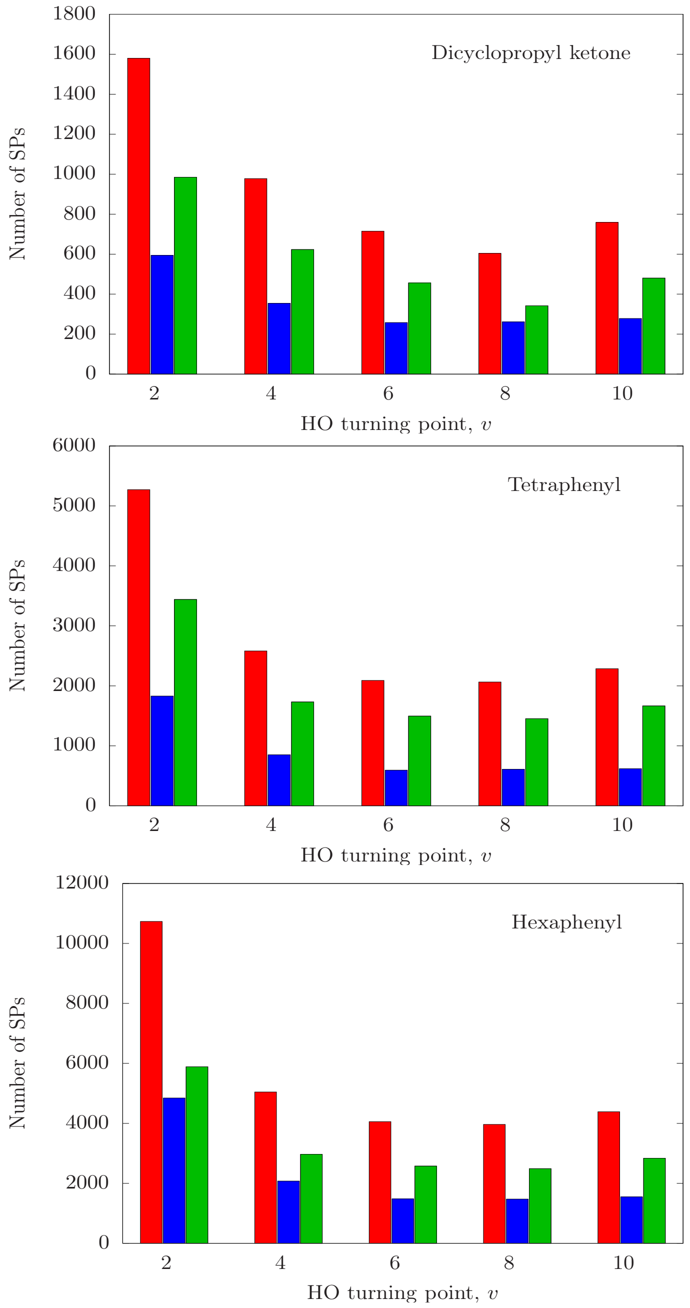


Figure S1: Number of SPs required for calculations of 1M2F PESs for dicyclopropyl ketone, tetraphenyl, and hexaphenyl using the DIF-ADGA employing different starting grid boundaries. Red bars show SPs for the entire set of vibrational modes, while blue and green bars represent SPs calculated along IC and INTRA modes, respectively.

## S2 Molecular Structures and Fragmentation Setup

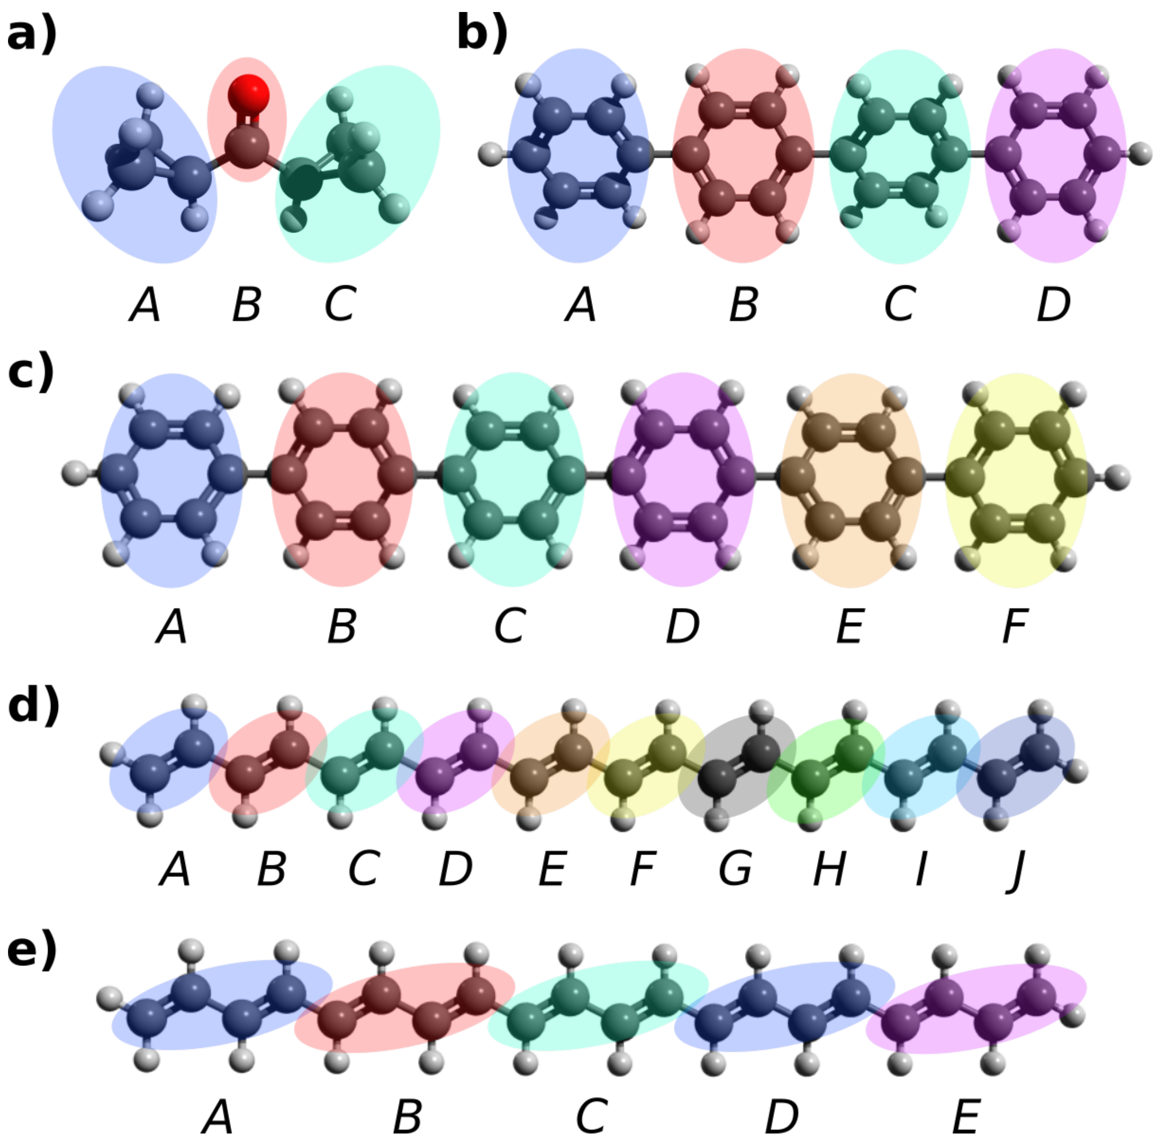


Figure S2: Molecular structures of a) dicyclopropyl ketone, b) tetraphenyl, c) hexaphenyl, and d)–e) icosadecaene. Colored ellipses show separate fragments used in creation of FCRs. Capital letters are used for fragment labeling. Two fragmentation schemes d) and e) are shown for the icosadecaene molecule.

# S3 Effective Fragment Combination Ranges

Table S1: Effective second order FCRs applied in PES construction for dicyclopropyl ketone, tetraphenyl, and hexaphenyl. For fragment labeling, see Fig. S1.

| |
|---|
| Dicyclopropyl ketone |
| $\{\{B\}, \{A, B\}, \{B, C\}\}$ |
| Tetraphenyl |
| $\{\{B\}, \{C\}, \{A, B\}, \{B, C\}, \{C, D\}\}$ |
| Hexaphenyl |
| $\{\{B\}, \{C\}, \{D\}, \{E\}, \{A, B\}, \{B, C\}, \{C, D\}, \{D, E\}, \{E, F\}\}$ |

Table S2: Effective FCRs of $l$th order used in PES construction for icosadecaene. The molecular system is fragmented to −CH=CH− units. For fragment labeling, see Fig. S1.

| $l$F | Effective FCR |
|---|---|
| 1F | $\{\{A\},\{B\},\{C\},\{D\},\{E\},\{F\},\{G\},\{H\},\{I\},\{J\}\}$ |
| 2F | $\{\{B\},\{C\},\{D\},\{E\},\{F\},\{G\},\{H\},\{I\},$ |
| | $\{A,B\},\{B,C\},\{C,D\},\{D,E\},\{E,F\},\{F,G\},\{G,H\},\{H,I\},\{I,J\}\}$ |
| 3F | $\{\{B,C\},\{C,D\},\{D,E\},\{E,F\},\{F,G\},\{G,H\},\{H,I\},$ |
| | $\{A,B,C\},\{B,C,D\},\{C,D,E\},\{D,E,F\},\{E,F,G\},\{F,G,H\},\{G,H,I\},\{H,I,J\}\ \}$ |
| 4F | $\{\{B,C,D\},\{C,D,E\},\{D,E,F\},\{E,F,G\},\{F,G,H\},\{G,H,I\},$ |
| | $\{A,B,C,D\},\{B,C,D,E\},\{C,D,E,F\},\{D,E,F,G\},\{E,F,G,H\},\{F,G,H,I\},\{G,H,I,J\}\}$ |
| 5F | $\{\{B,C,D,E\},\{C,D,E,F\},\{D,E,F,G\},\{E,F,G,H\},\{F,G,H,I\},$ |
| | $\{A,B,C,D,E\},\{B,C,D,E,F\},\{C,D,E,F,G\},\{D,E,F,G,H\},\{E,F,G,H,I\},\{F,G,H,I,J\}\}$ |
| 6F | $\{\{B,C,D,E,F\},\{C,D,E,F,G\},\{D,E,F,G,H\},\{E,F,G,H,I\},$ |
| | $\{A,B,C,D,E,F\},\{B,C,D,E,F,G\},\{C,D,E,F,G,H\},\{D,E,F,G,H,I\},\{E,F,G,H,I,J\}\}$ |
| 7F | $\{\{B,C,D,E,F,G\},\{C,D,E,F,G,H\},\{D,E,F,G,H,I\},$ |
| | $\{A,B,C,D,E,F,G\},\{B,C,D,E,F,G,H\},\{C,D,E,F,G,H,I\},\{D,E,F,G,H,I,J\}\}$ |
| 8F | $\{\{B,C,D,E,F,G,H\},\{C,D,E,F,G,H,I\},$ |
| | $\{A,B,C,D,E,F,G,H\},\{B,C,D,E,F,G,H,I\},\{C,D,E,F,G,H,I,J\}\}$ |
| 9F | $\{\{B,C,D,E,F,G,H,I\},$ |
| | $\{A,B,C,D,E,F,G,H,I\},\{B,C,D,E,F,G,H,I,J\}\}$ |

Table S3: Effective FCRs of $l$th order used in PES construction for icosadecaene. The molecular system is fragmented to $-(\mathrm{CH{=}CH})_2-$ units. For fragment labeling, see Fig. S1.

| $l$F | Effective FCR |
|---|---|
| 1F | $\{\{A\},\{B\},\{C\},\{D\},\{E\}\}$ |
| 2F | $\{\{B\},\{C\},\{D\},$ |
| | $\{A,B\},\{B,C\},\{C,D\},\{D,E\}\}$ |
| 3F | $\{\{B,C\},\{C,D\},$ |
| | $\{A,B,C\},\{B,C,D\},\{C,D,E\}\ \}$ |
| 4F | $\{\{B,C,D\},\{C,D,E\},$ |
| | $\{A,B,C,D\},\{B,C,D,E\}\}$ |
